# Supplementary material for: Gate-controlled analog memcapacitance in LaAlO3/SrTiO3 interface-based devices
Source: arXiv:2512.11176 source file (2025-12-11)
Supplement: Supplementary file 1 [file Supplementary.pdf]

## Supplementary Material:

### Gate-controlled analog memcapacitance in LAO/STO interface-based devices

Soumen Pradhan<sup>1, a</sup>, Victor Lopez-Richard<sup>2</sup>, Igor Ricardo<sup>2</sup>, Fabian Hartmann<sup>1, b</sup>, Ana Luiza Costa Silva<sup>2</sup>, Merit Spring<sup>1</sup>, Silke Kuhn<sup>1</sup>, Michael Sing<sup>1</sup>, Ralph Claessen<sup>1</sup> and Sven Höfling<sup>1</sup>

1) Julius-Maximilians-Universität Würzburg, Physikalisches Institut and Würzburg-Dresden Cluster of Excellence ct.qmat, Am Hubland, 97074 Würzburg, Deutschland

2) Department of Physics, Federal University of São Carlos, 13565-905 São Carlos, SP, Brazil

a) Electronic mail: soumen.pradhan@uni-wuerzburg.de

b) Electronic mail: fabian.hartmann@uni-wuerzburg.de

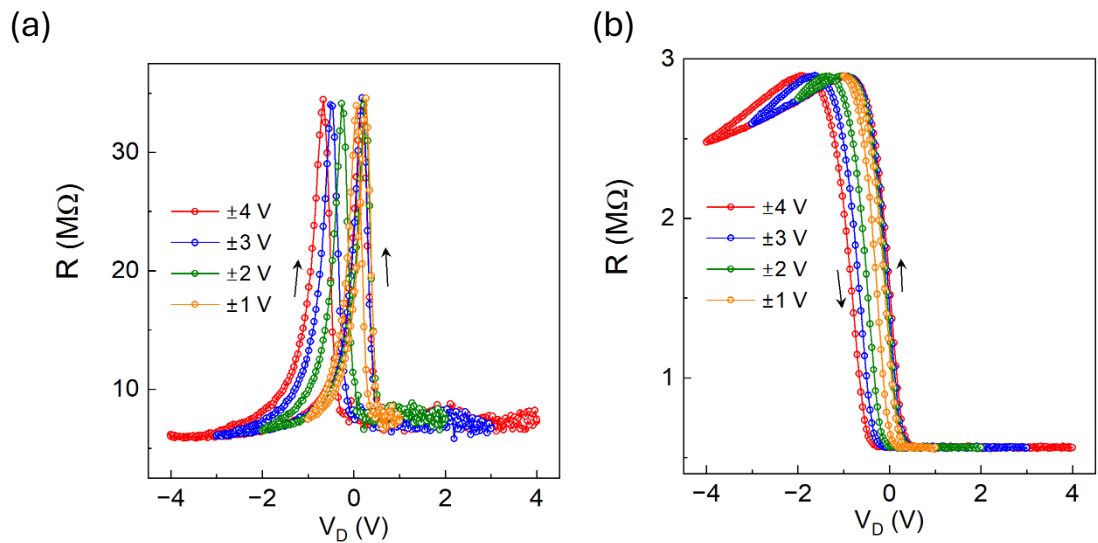

FIG. S1: Resistance-voltage hysteresis curves for different drain voltage ( $V_D$ ) amplitude with control gate at floating condition measured at ac voltage of frequency (a) 10 Hz and (b) 130 Hz as measured for memcapacitance measurements shown in Fig. 2(a) and 2(b).

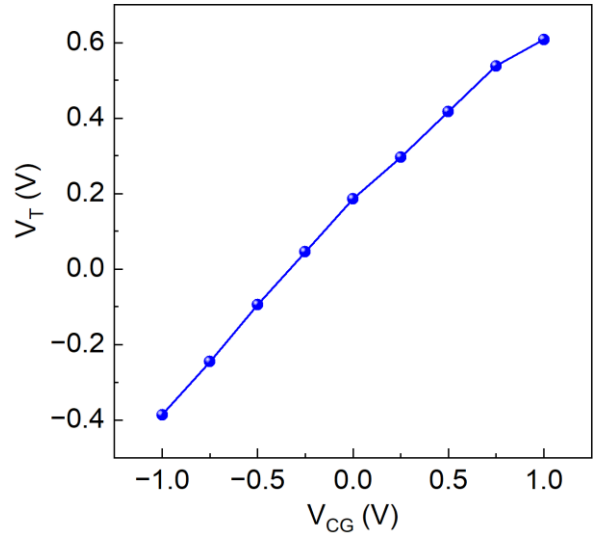

FIG. S2: Variation of threshold voltage ( $V_T$ ) with control gate voltage ( $V_{CG}$ ) extracted from Fig. 4(a) showing almost linear variation at negative  $V_{CG}$  and intend to saturate at positive  $V_{CG}$  with total tunability of approximately 1 V.

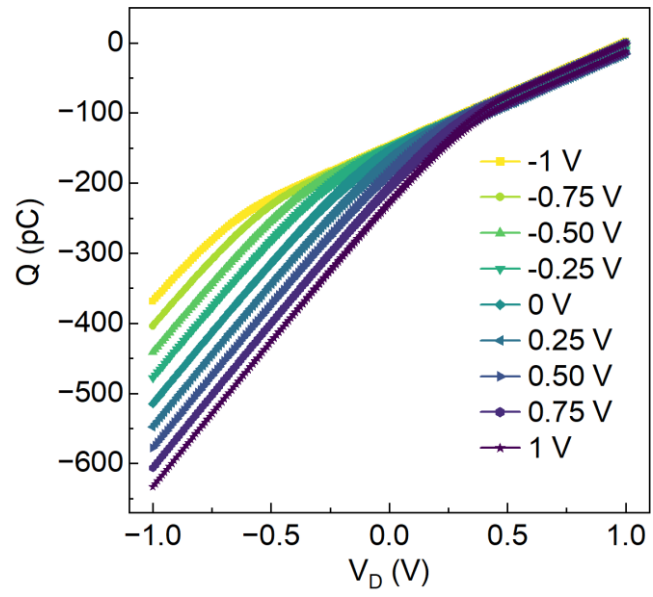

FIG. S3: Charge-voltage ( $Q$ - $V$ ) curves extracted from C-V curves in Fig. 4(a) for different  $V_{CG}$ .

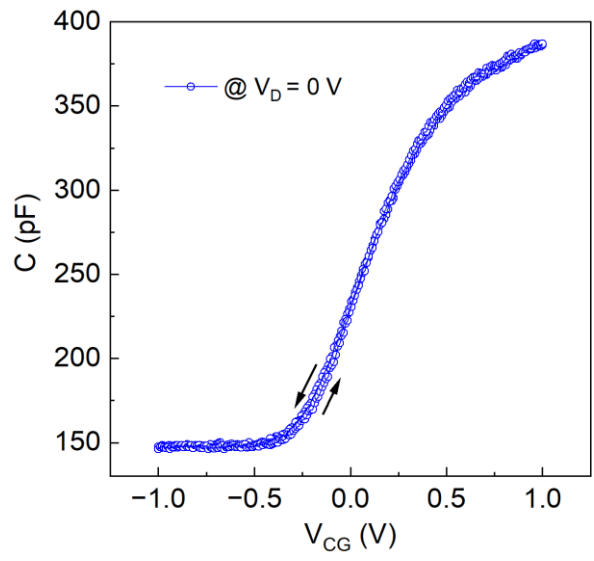

FIG. S4: Reversible gradual switching of capacitance with varying control gate voltage ( $V_{CG}$ ) at  $V_D=0$  V measured at an AC voltage of 10 Hz.
